# Supplementary material for: Nonlinear synchronization through vector subharmonic entrainment
Source: arXiv:2507.23596 source file (2025-07-31)
Supplement: Supplementary file 1 [file SupplementaryMaterialarxiv.pdf]

The EDF is subsequently spliced to the output port of a dual-stage polarization-sensitive optical isolator (ISO) with a center wavelength of 1550 nm and an extinction ratio of 28 dB. The 70/30 optical coupler (OC), featuring a coupling ratio centered at 1550 nm and an insertion loss around 1 dB, was employed to extract 30% of the laser power from the cavity. In addition, the configuration includes two fiber polarization controllers placed before and after the polarization-dependent optical isolator. The first one is the in-line miniature manual in-line polarization controller (PC). The second one is the electronic in-line polarization controller (EPC) with a three-section external voltage control. The EPC software enables full state-of-polarization control through thermal technology, ensuring stable polarization scanning across the entire Poincaré sphere. It is important to note that, except for the ISO and EDF, the full cavity of the laser was constructed using standard fiber SMF-28. The total fiber laser cavity length is 12.3 m comprising 0.2 m EDF, 1.5 m PM-1550 fiber, and 10.5 m of SMF-28 fiber. This length also includes pigtail fibers from the Electronic Polarization Controller (EPC), isolator, and coupler. The anomalous group velocity dispersion (GVD) values of the SMF-28 and PM-1550 fiber at 1.55  $\mu\text{m}$  were about  $-23 \text{ ps}^2/\text{km}$  and  $-22 \text{ ps}^2/\text{km}$ , respectively. The normal GVD of the Er-doped fiber at 1550 nm was estimated as  $15.3 \text{ ps}^2/\text{km}$ . As a result, the net dispersion of the cavity could be calculated as  $-0.27 \text{ ps}^2$ , suggesting that the laser was operating at an anomalous dispersion regime. For optical signal injection, a Polarization Scrambler (PS) EPS1000 (Novoplet) and a narrow linewidth continuous wave laser (CWL) CoBrite DX1 (IDPhotonics) with tunable wavelength are employed. The setup seeds an optical power of 15 dBm at 1.67 kHz through a vacant input port of a 30/70 output optical coupler. The output light pulses were characterized and analyzed using various detection and measurement techniques, including a 50 GHz High-Speed Photodetector, a real-time oscilloscope with 6 GHz bandwidth, and an optical spectrum analyzer AQ6317B (Yokogawa). A fast polarimeter PM1000-XL-FA-N20 D (Novoptel) with a sampling frequency of 100 MS/s to detect the evolution of the Stoke parameters  $S_1$ ,  $S_2$ ,  $S_3$ , and the total power  $S_0$ .

### **Liner stability analysis.**

By substituting  $u = |u|\exp(i \cdot \varphi_x)$  and  $v = |v|\exp(i \cdot \varphi_y)$  into Eqs. 3, we find the steady-state solution for the case of absence of the CW signal in the cavity, e. g.  $a = 0$  and  $(du/dt = dv/dt = df_1/dt = df_2/dt = df_3/dt = df_4/dt \equiv 0)$  as  $|u| = |v| = E_s$ ;

$\Delta\varphi = \varphi_y - \varphi_x = 0, \pi$ ;  $f_{2s} = 0$  from the equations:

$$\frac{\alpha_1}{1+\Delta^2} f_{1s} - \alpha_2 + A + \left( \frac{\alpha_1}{1+\Delta^2} f_{3s} + A \right) \cdot m = 0, a_1 f_{1s} + a_3 f_{3s} = b_1, \frac{a_3}{2} f_{1s} + a_1 f_{3s} = 0. \quad (\text{SE1})$$

Here

$$\begin{aligned} b_1 &= \frac{\chi^{-1}}{2} I_p - 1, a_1 = 1 + \frac{I_p}{2} + \frac{2\chi E_s^2}{1+\Delta^2}, a_3 = \frac{2\chi E_s^2 \cdot m}{1+\Delta^2}, \\ A_{11} &= A_{12} = A_{21} = A_{22} = A = -0.6931, m = \pm 1. \end{aligned} \quad (\text{SE2})$$

The results for  $E_s, f_{1s}, f_{3s}$  for  $m = \pm 1$  and  $\alpha_1 = 10.131, \varepsilon = 0.6 \cdot 10^{-5}, \alpha_2 = 2.3, \Delta = 0.015, \chi = 2.3, \gamma = 2 \cdot 10^{-6}, \delta = 1$  and  $a = 0$  are shown in Fig. 6 (a).

For linear stability analysis, we substitute the following ansatz into Eqs. (5):

$$\mathbf{F}(t) \equiv \begin{pmatrix} |u| \\ |v| \\ \Delta\varphi \\ f_1 \\ f_2 \\ f_3 \end{pmatrix} = \begin{pmatrix} E_s \\ E_s \\ 0 (\pi) \\ f_{1s} \\ 0 \\ f_{3s} \end{pmatrix} + \begin{pmatrix} x_0 \\ x_1 \\ x_2 \\ x_3 \\ x_4 \\ x_5 \end{pmatrix} \cdot \exp(\lambda t), \quad (\text{SE3})$$

and find the following equation for eigenvalues:

$$\det \begin{bmatrix} k_1 - \lambda & k_2 m & k_3 m & k_4 & k_4 & k_4 \cdot m \\ k_2 m & k_1 - \lambda & -k_3 \cdot m & k_4 & -k_4 & k_4 \cdot m \\ -k_5 \cdot m & k_5 \cdot m & -2k_2 m - \lambda & 0 & -k_6 m & 0 \\ -k_7 & -k_7 & 0 & -k_8 - \lambda & 0 & -k_9 \\ -k_{10} & k_{10} & 0 & 0 & -k_8 - \lambda & 0 \\ -k_{11} & -k_{11} & 0 & \frac{-k_9}{2} & 0 & -k_8 - \lambda \end{bmatrix} \equiv 0. \quad (\text{SE4})$$

Here

$$\begin{aligned} k_1 &= \frac{\alpha_1}{1+\Delta^2} f_{1s} - \alpha_2 + A, k_2 = \frac{\alpha_1}{1+\Delta^2} f_{3s} + A, k_3 = \frac{\alpha_1 \Delta}{1+\Delta^2} f_{3s} E_s, k_4 = \frac{\alpha_1}{1+\Delta^2} E_s, \\ k_5 &= \frac{2\alpha_1 \Delta}{1+\Delta^2} \frac{f_{3s}}{E_s}, k_6 = \frac{2\alpha_1 \Delta}{1+\Delta^2}, k_7 = \frac{2\chi \cdot \varepsilon \cdot E_s}{1+\Delta^2} (f_{1s} + f_{3s} \cdot m), \\ k_8 &= a_1 = \varepsilon \cdot \left( 1 + \frac{I_p}{2} + \frac{2\chi E_s^2}{1+\Delta^2} \right), k_9 = \frac{2\varepsilon \cdot \chi E_s^2}{1+\Delta^2} m, \\ k_{10} &= \frac{\chi \cdot \varepsilon \cdot E_s f_{1s}}{1+\Delta^2}, k_{11} = \frac{\chi \cdot \varepsilon \cdot E_s}{1+\Delta^2} (f_{1s} \cdot m + 2f_{3s}). \end{aligned} \quad (\text{SE5})$$

As a result, Eq. (SE4) takes the following form:

$$(2\lambda^3 + c_1 \lambda^2 + c_2 \lambda + c_3) \cdot (\lambda^3 + d_1 \lambda^2 + d_2 \lambda + d_3) \equiv 0. \quad (\text{SE6})$$

Here

$$c_1 = 4k_8 - 2k_1 - 2k_2 m,$$

$$\begin{aligned}
c_2 &= 2k_8^2 - 4k_8(k_1 + k_2) - (k_9^2 - 4k_4(k_7 + k_{11}m)), \\
c_3 &= (k_9^2 - 2k_8^2)(k_1 + k_2m) - 2k_4k_9(2k_{11} + k_7m) + 4k_4k_8(k_7 + k_{11}m), \\
d_1 &= k_8 - k_1 + 3k_2m, \\
d_2 &= 2k_2^2 + k_2m(3k_8 - 2k_1) + 2k_3k_5 - k_1k_8m + 2k_4k_{10}m, \\
d_3 &= 2k_8(k_2^2 - k_1k_2m + k_3k_5) + 2k_{10}(2k_2k_4m - k_3k_6). \quad (\text{SE7})
\end{aligned}$$

For the following parameters:  $\alpha_1 = 10.131$ ,  $\varepsilon = 0.6 \cdot 10^{-5}$ ,  $\alpha_2 = 2.3$ ,  $\Delta = 0.015$ ,  $\chi = 2.3$ ,  $\gamma = 2 \cdot 10^{-6}$ ,  $\delta = 1$  and  $a = 0$  (no injected signal), the eigenvalue split in two branches:

$$\begin{aligned}
(I) \quad \lambda_0 &= R_0, \quad \lambda_{1,2} = R_1 \pm i\Omega_{1,2}, \quad (II) \quad \lambda_3 = R_2, \quad \lambda_{4,5} = R_3 \pm i\Omega_{3,4} \\
R_0 &< 0, \quad R_1 < 0, \quad R_2 < 0 \quad (\Delta\varphi = 0), \quad R_2 > 0 \quad (\Delta\varphi = \pi), \quad R_3 > 0.
\end{aligned}$$

(SE8)

All eigenvalues with negative real part, e. g.  $\lambda_0 - \lambda_3$ , are shown in Fig. 2S.

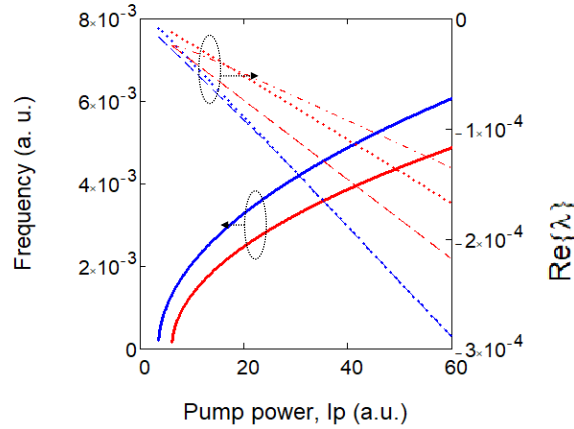

FIG. 2S (color online) Steady-state stability analysis of NPR-mode locked laser without CW signal in the laser cavity. Eigenvalues with negative real parts as a function of the pump power  $I_p$ ,  $\Delta\varphi = 0$  (red lines),  $\Delta\varphi = \pi$  (blue lines);  $\Omega_{1,2}$  (solid lines);  $R_1$  (dotted lines);  $R_0$  (dashed lines),  $R_0$  (dash-dotted line).
